# Supplementary material for: Accurate real-time evolution of electron densities and ground-state properties from generalized Kohn-Sham theory
Source: arXiv:1909.02510 source file (2020-01-11)

In [1]:
```
%matplotlib inline
import warnings
warnings.filterwarnings('ignore')
#import matplotlib
#matplotlib.use('Agg')
```

# 1. Designing the model $H_2$ molecule

## 1.1. Determining the softening parameters for H atoms in iDEA

In order to closely approach a real $H_2$ molecule in iDEA we need to use appropriate softening parameters. There are two such parameters, one for the electrons ($\alpha$)

$$V_e(x) = \frac{1}{|x| + \alpha},$$

and one for the protons ($\beta$)

$$V_p(x) = \frac{1}{|x| + \beta}.$$

As shown in M.J.P Hodgson's thesis (https://www.researchgate.net/publication/333760017_Electrons_in_model_nanostructures) (Appendinx A.2) to model as closely as possibly the interaction of two charged disks the appropriate electron softening parameter is:

$$\alpha = 1.0$$

Now we will determine the value of $\beta$. To determine it we will compute the total energy of a one-electron atom with the following external potential:

$$V_{ext}(x) = \frac{1}{|x| + \beta}.$$

As we want to converge the scale of $\beta$ will write it as:

$$V_{ext}(x) = \frac{1}{|x| + 10^{-b}}.$$

And then plot $E(b)$ to see what value of $b$ gives the correct value of the ground-state energy $E = -13.6$eV.

This in $E = -0.5$ (a.u) in atomic units.

In [2]:
```
E_target = -0.5
```

First lets just try $b = 0$:

In [3]:
```
# import all needed modules
import numpy as np
import scipy as sp
import matplotlib.pyplot as plt
plt.rc('text', usetex=True) # use LaTeX
from iDEA.input import Input
```

In [4]:
```
# set up the system
pm = Input()
pm.sys.NE = 1 # number of electrons
pm.sys.grid = 1001 # number of grid points
pm.sys.xmax = 10.0 # lenght of system L = 2*xmax
pm.sys.acon = 1.0 # the value of alpha
pm.run.name = 'h_atom'

b = 0
def v(x):
    return -1.0/(abs(x)+10**-b) # the value of beta=10^-b

pm.setup_space()
pm.run.setup_space = False
pm.space.v_ext = np.copy(v(pm.space.grid)) # set the external potential
```

In [5]:
```
# use EXT1 to find exact energy
import iDEA.EXT1
pm.make_dirs()
pm.check()
result = iDEA.EXT1.main(pm)
```

```
EXT: constructing arrays
EXT: solving the time-independent Schrodinger equation
EXT: calculated the ground-state
E0 = -0.50003
```

We can plot the external potential and ground-state charge density:

In [6]:
```
# plot n and Vext for b=0
x = pm.space.grid
plt.plot(x, result.gs_ext_den, linewidth=2, linestyle='-', color='k', label='$n$')
plt.plot(x, result.gs_ext_vxt, linewidth=2, linestyle='-.', color='b', label='$V_{\mathrm{ext}}$')

# configure and save plot
plt.legend(frameon=False)
plt.xlabel(r'$x$ (a.u.)', size=25)
plt.ylabel(r'$n$, $V_{\mathrm{ext}}$ (a.u.)', size=25)
plt.tick_params(top='on', right='on')
plt.tick_params(direction='in')
plt.gcf().subplots_adjust(left=0.18)
plt.gcf().subplots_adjust(bottom=0.18)
plt.savefig('h_atom.pdf')
```

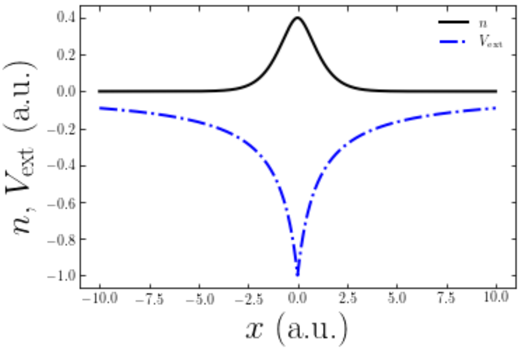


So this value already gives a remarkably close energy to the target energy with an absolute error of:

In [7]:
```
E_error = abs(E_target - result.gs_ext_E)
print('E_error = {} a.u.'.format(E_error))
```

```
E_error = 2.649331748516559e-05 a.u.
```

To make sure this isnt a fluke lets loop over $b$ to find the best $b$:

In [8]:
```
pm.run.verbosity = 'low'
b_list = [0.0, 1.0, 2.0, 3.0, 4.0, 5.0, 6.0]
E_list = []
error_list = []
for i in range(0, len(b_list)):
    b = b_list[i]
    pm.space.v_ext = np.copy(v(pm.space.grid)) # set the external potential
    result = iDEA.EXT1.main(pm)
    E_list.append(result.gs_ext_E)
    error_list.append(abs(E_target - result.gs_ext_E))
    print('b = {0}, E = {1}, error = {2}'.format(b_list[i], E_list[i], error_list[i]))
```

```
b = 0.0, E = -0.5000264933174852, error = 2.649331748516559e-05
b = 1.0, E = -2.731216456804313, error = 2.231216456804313
b = 2.0, E = -12.371601413503075, error = 11.871601413503075
b = 3.0, E = -196.0966496559424, error = 195.5966496559424
b = 4.0, E = -7099.571324878994, error = 7099.071324878994
b = 5.0, E = -96364.72964351634, error = 96364.22964351634
b = 6.0, E = -996280.9352739787, error = 996280.4352739787
```

So we know the value of $\beta$ is about $10^0 = 1.0$ lets now search in the region of 1 (from 0.5 to 1.5):

In [9]:
```
def v(x):
    return -1.0/(abs(x)+beta) # the value of beta

pm.run.verbosity = 'low'
beta_list = [0.5, 0.6, 0.7, 0.8, 0.9, 1.0, 1.1, 1.2, 1.3, 1.4, 1.5]
E_list = []
error_list = []
for i in range(0, len(beta_list)):
    beta = beta_list[i]
    pm.space.v_ext = np.copy(v(pm.space.grid)) # set the external potential
    result = iDEA.EXT1.main(pm)
    E_list.append(result.gs_ext_E)
    error_list.append(abs(E_target - result.gs_ext_E))
    print('beta = {0}, E = {1}, error = {2}'.format(beta_list[i], E_list[i], error_list[i]))
```

```
beta = 0.5, E = -0.8599751320147521, error = 0.35997513201475206
beta = 0.6, E = -0.7474941859981934, error = 0.2474941859981934
beta = 0.7, E = -0.6630304287465941, error = 0.16303042874659412
beta = 0.8, E = -0.5970182718802778, error = 0.09701827188027778
beta = 0.9, E = -0.5438550104246869, error = 0.04385501042468687
beta = 1.0, E = -0.5000264933174852, error = 2.649331748516559e-05
beta = 1.1, E = -0.4632095864743265, error = 0.036790413525673527
beta = 1.2, E = -0.4318031043699955, error = 0.06819689563000447
beta = 1.3, E = -0.40466535815017773, error = 0.09533464184982227
beta = 1.4, E = -0.3809590292770049, error = 0.11904097072299508
beta = 1.5, E = -0.36005524621511764, error = 0.13994475378488236
```

Plotting the error in $E$ against $\beta$:

In [10]:
```
# plot E vs beta
plt.plot(beta_list, error_list, linewidth=2, linestyle='-', color='k')

# configure and save plot
plt.xlabel(r'$\beta$ (a.u.)', size=25)
plt.ylabel(r'$E_{\mathrm{error}}$ (a.u.)', size=25)
plt.tick_params(top='on', right='on')
plt.tick_params(direction='in')
plt.gcf().subplots_adjust(left=0.18)
plt.gcf().subplots_adjust(bottom=0.18)
plt.savefig('softening.pdf')
```

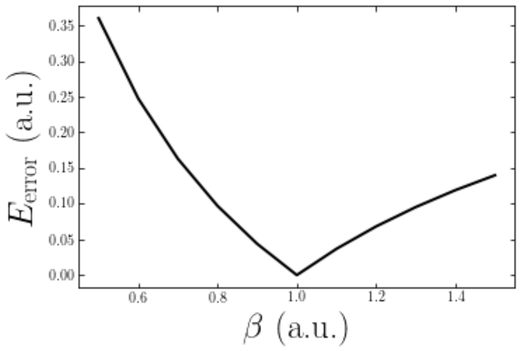


So the final values are: $\alpha = 1.0$ and $\beta = 1.0$, in iDEA these give the value of the energy of out model hydrogen atom to be: $E = -13.6$eV.

## 1.2 Testing our model Hydrogen molecule

Here we will investgate a model $\mathrm{H}_2$ molecule to see if a convelent bond forms between a system of two opposite-spin electron system comprised or two proton wells seperated by a distance $d$. We will plot the total energy $E = E_\mathrm{e} + E_\mathrm{p}$ against distance $d$.

We will use this curve to measure the:

- bond length
- bond energy
- enthalpy of formation
- dissociation energy
- total energy at bond length

We will then compare these measurments in iDEA against the experimental values for $\mathrm{H}_2$ to see how closely our model system in iDEA encapsulates the physics of a real $\mathrm{H}_2$ molecule.

We will calculate $E(d)$ for $\mathrm{H}_2$ to determine the bond length:

In [11]:
```
# set up the system
pm = Input()
pm.run.name = 'h2_test'
pm.sys.NE = 2 # number of electrons
pm.sys.spin = 'opposite' # both electrons treated as opposite spin
pm.sys.grid = 501
pm.sys.xmax = 10.0
pm.sys.acon = 1.0   # value of alpha (see section 1.1)
beta = 1.0          # value of beta (see section 1.1)
pm.setup_space()
pm.run.setup_space = False
```

To make sure the system is wide enouph let's plot the external potential at the maximum width (8.0 a.u):

In [12]:
```
d = 8.0
def v(x):
    return -1.0/(np.abs(x+0.5*d)+beta)-1.0/(np.abs(x-0.5*d)+beta)
x = np.linspace(-pm.sys.xmax, pm.sys.xmax, pm.sys.grid)
dx = x[1] - x[0]
plt.plot(x, v(x), linestyle='-', color='k')

# configure and save plot
plt.xlabel(r'$x$ (a.u.)', size=25)
plt.ylabel(r'$V_{\mathrm{ext}}$ (a.u.)', size=25)
plt.tick_params(top='on', right='on')
plt.tick_params(direction='in')
plt.gcf().subplots_adjust(left=0.18)
plt.gcf().subplots_adjust(bottom=0.18)
plt.savefig('v.pdf')
```

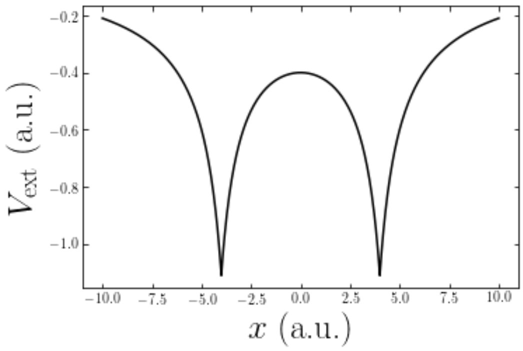


In [13]:
```
# make array of distances
ds = np.linspace(0.0, 8.0, 60)
```

In [14]:
```
# WARNING: Long Run! Does not need to be run again for rest of the script to work!

# main loop, stretching the molecule from 0 to 8 a.u
for i in range(ds.shape[0]):
    d = ds[i]
    print('running d={0}'.format(d))
    pm.run.name = 'h2_{0}'.format(i)
    pm.space.v_ext = np.copy(v(x)) # set the external potential
    pm.make_dirs()
    pm.run.verbosity = 'low'
    result = iDEA.EXT2.main(pm)
```

In [15]:
```
# load in energies and distances
E_list = []
for i in range(ds.shape[0]):
    E = pickle.load(open('outputs/h2_{0}/raw/gs_ext_E.db'.format(i),'rb'))
    E_list.append(E)

# convert to numpy arrays
E_e = np.array(E_list)

# add in proton energy
E_p = 1.0/(np.abs(ds)+beta)
E = E_e + E_p
```

In [16]:
```
# plot energy curve
plt.axhline(y=-1.0, xmin=0.0, xmax=8.2, linewidth=1, color = 'k')
plt.plot(ds, E, linestyle='-', color='k', linewidth=2)

# configure and save plot
plt.xlabel(r'$d$ (a.u.)', size=25)
plt.ylabel(r'$E$ (a.u.)', size=25)
plt.tick_params(top='on', right='on')
plt.tick_params(direction='in')
plt.gcf().subplots_adjust(left=0.18)
plt.gcf().subplots_adjust(bottom=0.18)
plt.savefig('exact_h2.pdf')
```

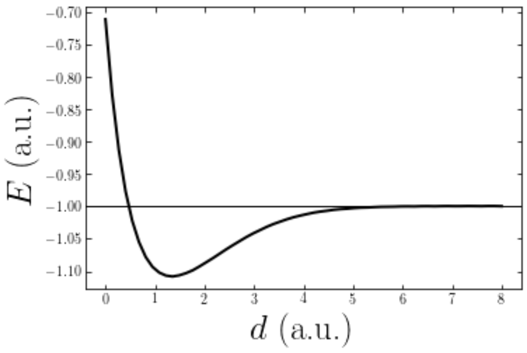


We will now use this curve to measure the bond length:

In [17]:
```
bond_length = ds[E.argmin()]
bond_error = ds[1] - ds[0]
d_target = 1.398 # experimental bond length in a.u.
percent_error = (abs(bond_length - d_target)/d_target)*100.0
print('bond length = {0:.3f} +/- {1:.3f}'.format(bond_length, bond_error))
print('experimental bond length = {}'.format(d_target))
print(r'error = {:.0f}%'.format(percent_error))
```

```
bond length = 1.356 +/- 0.136
experimental bond length = 1.398
error = 3%
```

To determine the bond energy we simply need to take the absolute difference between the energy at the bond length and the energy at total dissociation. The experimental value is 4.510 eV.

In [18]:
```
natural_energy = np.min(E)
stretched_energy = E[-1] # from bond curve
bond_energy = abs(stretched_energy - natural_energy)
bond_target = 4.510 / 27.211385  # experimental bond energy in a.u.
percent_error = (abs(bond_energy - bond_target)/bond_target)*100.0
print('bond energy = {0:.3f}'.format(bond_energy))
print('experimental bond energy = {0:.3f}'.format(bond_target))
print(r'error = {:.0f}%'.format(percent_error))
```

```
bond energy = 0.108
experimental bond energy = 0.166
error = 35%
```

The energy of formation is the ammount of energy released during the formation of a $\mathrm{H_2}$ molecule:

$$\mathrm{H} + \mathrm{H} \rightarrow \mathrm{H_2}$$

This energy is negative when forming the bond, and positive when breaking the bond. For $\mathrm{H_2}$ this is simply given by the negative of the bond energy.

In [19]:
```
formation = -bond_energy
formation_target = -bond_target  # experimental value in a.u.
percent_error = (abs(formation - formation_target)/(-formation_target)*100.0)
print('enthalpy of formation = {0:.3f}'.format(formation))
print('experimental enthalpy of formation = {0:.3f}'.format(formation_target))
print(r'error = {:.0f}%'.format(percent_error))
```

```
enthalpy of formation = -0.108
experimental enthalpy of formation = -0.166
error = 35%
```

The dissociation energy is taken as the energy as the bond is stretched apart to infinity. The experimental value of this is 1.0 a.u.

In [20]:
```
dissociation = E[-1]
dissociation_target = -1.0000  # experimental value in a.u.
percent_error = (abs(dissociation - dissociation_target)/(-dissociation_target)*100.0)
print('dissociation energy = {0:.3f}'.format(dissociation))
print('experimental dissociation energy = {0:.3f}'.format(dissociation_target))
print(r'error = {:.0f}%'.format(percent_error))
```

```
dissociation energy = -1.000
experimental dissociation energy = -1.000
error = 0%
```

The total energy (eletrons only) at the bond length is the usual energy obtained from the Schrodinger equation. In order to deremine the experimantal we will take off the proton energy:

In [21]:
```
electron = E_e[E.argmin()]                      # electron energy at bond length
target_total = -1.166                           # experimental total energy at bond length in a.u.
target_distance = 1.398                         # experimental bond length in a.u.
target_proton = 1.0/target_distance             # experimental proton energy at bond length in a.u.
target_electron = target_total - target_proton  # experimental electron energy at bond length in a.u.

percent_error = (abs(electron - target_electron)/(-target_electron)*100.0)
print('total (electron) energy at bond length = {0:.3f}'.format(electron))
print('experimantal total (electron) energy at bond length = {0:.3f}'.format(target_electron))
print(r'error = {:.0f}%'.format(percent_error))
```

```
total (electron) energy at bond length = -1.533
experimantal total (electron) energy at bond length = -1.881
error = 19%
```

In summary, the model we have developed in iDEA is very satifactory of capturing the physics of the real hydrogen molecule. We can now begin testing existing and novel approximations using this as the model test system.

| Property | iDEA | Experimental | Error |
|---|---|---|---|
| Bond length | 1.356 | 1.398 | 3% |
| Bond energy | 0.108 | 0.166 | 35% |
| Enthalpy of formation | -0.108 | -0.166 | 35% |
| Dissociation energy | -1.000 | -1.000 | 0% |
| Total energy | -1.531 | -1.881 | 19% |

# 2. Exact and approximate energy dissociation curves

We will now compare each of our approximate methods (RHF, RDA+, UHF, ULDA+) against the exact dissociation curves for our model hydrogen molecule:

In [22]:
```
# imports iDEA modules
import iDEA.RHF
import iDEA.UHF
import iDEA.RLDAp
import iDEA.ULDAp

# allow HF and LDA+ methods to converge for large streched limit
pm.hf.con = 1e-10
pm.ldap.con = 1e-10
```

In [23]:
```
# WARNING: Long Run! Does not need to be run again for rest of the script to work!

# main loop, stretching the molecule from 0 to 8 a.u
for i in range(ds.shape[0]):
    d = ds[i]
    print('running d={0}'.format(d))
    pm.run.name = 'h2_{0}'.format(i)
    pm.space.v_ext = np.copy(v(x)) # set the external potential
    if i > 44: # change the mixing parameter for the large distances for stability
        pm.hf.nu = 0.1
        pm.ldap.nu = 0.1
    result_rhf = iDEA.RHF.main(pm)
    result_uhf = iDEA.UHF.main(pm)
    result_rldap = iDEA.RLDAp.main(pm)
    result_uldap = iDEA.ULDAp.main(pm)
```

In [24]:
```
# load in energies and distances
E_rhf = []
E_uhf = []
E_rldap = []
E_uldap = []
for i in range(ds.shape[0]):
    E0 = pickle.load(open('outputs/h2_{0}/raw/gs_rhf_E.db'.format(i),'rb'))
    E_rhf.append(E0)
    E0 = pickle.load(open('outputs/h2_{0}/raw/gs_uhf_E.db'.format(i),'rb'))
    E_uhf.append(E0)
    E0 = pickle.load(open('outputs/h2_{0}/raw/gs_rldap_E.db'.format(i),'rb'))
    E_rldap.append(E0)
    E0 = pickle.load(open('outputs/h2_{0}/raw/gs_uldap_E.db'.format(i),'rb'))
    E_uldap.append(E0)

# convert to numpy arrays
E_rhf = np.array(E_rhf)
E_uhf = np.array(E_uhf)
E_rldap = np.array(E_rldap)
E_uldap = np.array(E_uldap)

# add in proton energy
E_p = 1.0/(np.abs(ds)+beta)
E_rhf += E_p
E_uhf += E_p
E_rldap += E_p
E_uldap += E_p
```

In [25]:
```
# plot energy curve
plt.axhline(y=-1.0, xmin=0.0, xmax=8.2, linewidth=1, color = 'k')
plt.plot(ds, E, linestyle='-', dashes=(), color='k', linewidth=2, label='Exact')
plt.plot(ds, E_rhf, linestyle='--', dashes=(3, 3), color='red', linewidth=2, label='RHF')
plt.plot(ds, E_uhf, linestyle='--', dashes=(1, 1), color='lime', linewidth=2, label='UHF')
plt.plot(ds, E_rldap, linestyle='--', dashes=(3,1,1,1), color='darkviolet', linewidth=2, label='RLDA+')
plt.plot(ds, E_uldap, linestyle='--', dashes=(0.5,0.5), color='cyan', linewidth=2, label='ULDA+')

# configure and save plot
plt.legend(frameon=False)
plt.xlabel(r'$d$ (a.u.)', size=25)
plt.ylabel(r'$E$ (a.u.)', size=25)
plt.tick_params(top='on', right='on')
plt.tick_params(direction='in')
plt.gcf().subplots_adjust(left=0.18)
plt.gcf().subplots_adjust(bottom=0.18)
plt.savefig('h2.pdf')
```

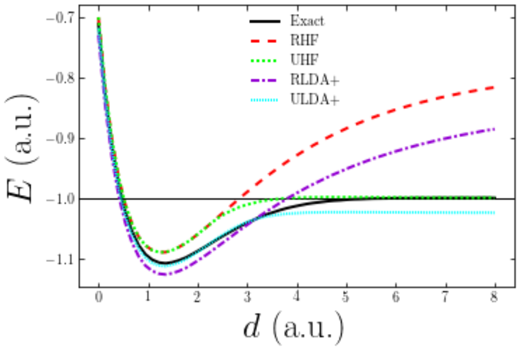


## 3. Charge density at natural length

We will now compare the accuracy of the charge density of each of the approximate methods at the molecules natural length:

In [26]:
```
# system the natural length
d = ds[E.argmin()]
i = E.argmin()
pm.space.v_ext = np.copy(v(x)) # set the external potential

# load in the densities
n = pickle.load(open('outputs/h2_{0}/raw/gs_ext_den.db'.format(i),'rb'))
n_rhf = pickle.load(open('outputs/h2_{0}/raw/gs_rhf_den.db'.format(i),'rb'))
n_uhf = pickle.load(open('outputs/h2_{0}/raw/gs_uhf_den.db'.format(i),'rb'))
n_rldap = pickle.load(open('outputs/h2_{0}/raw/gs_rldap_den.db'.format(i),'rb'))
n_uldap = pickle.load(open('outputs/h2_{0}/raw/gs_uldap_den.db'.format(i),'rb'))
```

In [27]:
```
# plot densities
plt.plot(x, n, linestyle='-', dashes=(), color='k', linewidth=2, label='Exact')
plt.plot(x, n_rhf, linestyle='--', dashes=(3, 3), color='red', linewidth=2, label='RHF')
plt.plot(x, n_rldap, linestyle='--', dashes=(3,1,1,1), color='darkviolet', linewidth=2, label='RLDA+')
plt.plot(x, n_uhf, linestyle='--', dashes=(1, 1), color='lime', linewidth=2, label='UHF')
plt.plot(x, n_uldap, linestyle='--', dashes=(0.5,0.5), color='cyan', linewidth=2, label='ULDA+')

# configure and save plot
plt.legend(frameon=False)
plt.xlabel(r'$x$ (a.u.)', size=25)
plt.ylabel(r'$n$ (a.u.)', size=25)
plt.tick_params(top='on', right='on')
plt.tick_params(direction='in')
plt.gcf().subplots_adjust(left=0.18)
plt.gcf().subplots_adjust(bottom=0.18)
plt.savefig('h2_natural.pdf')
```

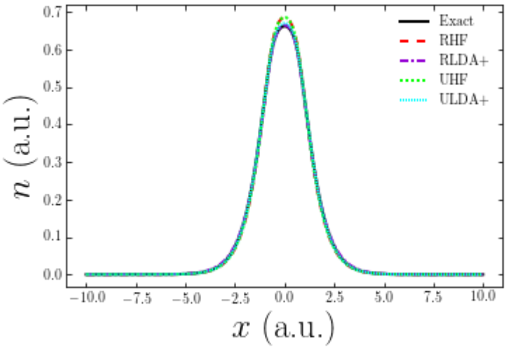


# 4. Charge density at stretched (dissociated) length

We will now compare the accuracy of the charge density of each of the approximate methods at the molecules stretched (dissociated) length:

In [28]:
```
# system the stretched length
d = ds[-1]
i = 59
pm.space.v_ext = np.copy(v(x)) # set the external potential

# load in the densities
n = pickle.load(open('outputs/h2_{0}/raw/gs_ext_den.db'.format(i),'rb'))
n_rhf = pickle.load(open('outputs/h2_{0}/raw/gs_rhf_den.db'.format(i),'rb'))
n_uhf = pickle.load(open('outputs/h2_{0}/raw/gs_uhf_den.db'.format(i),'rb'))
n_rldap = pickle.load(open('outputs/h2_{0}/raw/gs_rldap_den.db'.format(i),'rb'))
n_uldap = pickle.load(open('outputs/h2_{0}/raw/gs_uldap_den.db'.format(i),'rb'))
```

In [29]:
```
# plot densities
plt.plot(x, n, linestyle='-', dashes=(), color='k', linewidth=2, label='Exact')
plt.plot(x, n_rhf, linestyle='--', dashes=(3, 3), color='red', linewidth=2, label='RHF')
plt.plot(x, n_rldap, linestyle='--', dashes=(3,1,1,1), color='darkviolet', linewidth=2, label='RLDA+')
plt.plot(x, n_uhf, linestyle='--', dashes=(1, 1), color='lime', linewidth=2, label='UHF')
plt.plot(x, n_uldap, linestyle='--', dashes=(0.5,0.5), color='cyan', linewidth=2, label='ULDA+')

# configure and save plot
plt.legend(frameon=False)
plt.xlabel(r'$x$ (a.u.)', size=25)
plt.ylabel(r'$n$ (a.u.)', size=25)
plt.tick_params(top='on', right='on')
plt.tick_params(direction='in')
plt.gcf().subplots_adjust(left=0.18)
plt.gcf().subplots_adjust(bottom=0.18)
plt.savefig('h2_stretched.pdf')
```

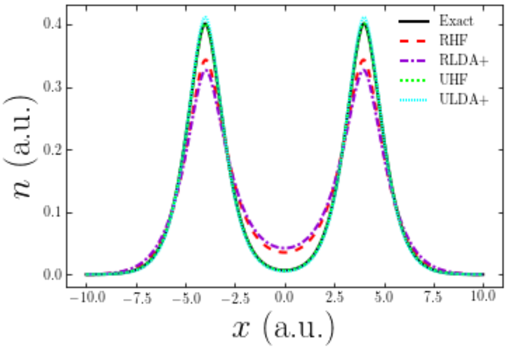

# 5. Time-dependence of charge density at natural length due to external electric field

We will now apply a uniform electic field across our model hydrogen molecule, and compare our approximxate methods to the exact real time evolving density:

In [30]:
```
# system the natural length
d = ds[E.argmin()]
i = E.argmin()
print('i of natural length = {0}'.format(i))
pm.space.v_ext = np.copy(v(x)) # set the external potential
pm.run.name = 'h2_{0}'.format(i)
pm.run.verbosity = 'default'

# set-up parameters for time dependence:
def vp(x):
    return -0.03*x # electric field of strength 0.08 a.u.
pm.sys.v_pert = vp
pm.setup_space()
pm.space.v_ext = np.copy(v(x)) # set the external potential
pm.run.time_dependence = True
pm.sys.tmax = 30.0 # Total real time
pm.sys.imax = 3001 # Number of real time iterations
```

```
i of natural length = 10
```

In [31]:
```
# WARNING: Long Run! Does not need to be run again for rest of the script to work!

# run the system with exact and approximate methods
pm.run.verbosity = 'default'
result_ext = iDEA.EXT2.main(pm)
result_uhf = iDEA.UHF.main(pm)
result_rhf = iDEA.RHF.main(pm)
result_uldap = iDEA.ULDAp.main(pm)
result_rldap = iDEA.RLDAp.main(pm)
```

In [32]:
```
# import densities
n_ext = pickle.load(open('outputs/h2_{0}/raw/td_ext_den.db'.format(i),'rb'))
n_uhf = pickle.load(open('outputs/h2_{0}/raw/td_uhf_den.db'.format(i),'rb'))
n_rhf = pickle.load(open('outputs/h2_{0}/raw/td_rhf_den.db'.format(i),'rb'))
n_uldap = pickle.load(open('outputs/h2_{0}/raw/td_uldap_den.db'.format(i),'rb'))
n_rldap = pickle.load(open('outputs/h2_{0}/raw/td_rldap_den.db'.format(i),'rb'))

# compute errors in the densities as a function of time
t = np.linspace(0.0, pm.sys.tmax, pm.sys.imax)
error_uhf = np.zeros(shape=pm.sys.imax)
error_rhf = np.zeros(shape=pm.sys.imax)
error_uldap = np.zeros(shape=pm.sys.imax)
error_rldap = np.zeros(shape=pm.sys.imax)
for i in range(pm.sys.imax):
    error_uhf[i] = np.sum(abs(n_ext[i,:] - n_uhf[i,:]))*dx
    error_rhf[i] = np.sum(abs(n_ext[i,:] - n_rhf[i,:]))*dx
    error_uldap[i] = np.sum(abs(n_ext[i,:] - n_uldap[i,:]))*dx
    error_rldap[i] = np.sum(abs(n_ext[i,:] - n_rldap[i,:]))*dx
```

In [33]:

```
# plot error curves
plt.plot(t, error_rhf, linestyle='--', dashes=(3, 3), color='red', linewidth=2, label='RHF')
plt.plot(t, error_rldap, linestyle='--', dashes=(3,1,1,1), color='darkviolet', linewidth=2, label='RLDA+')
plt.plot(t, error_uhf, linestyle='--', dashes=(1, 1), color='lime', linewidth=2, label='UHF')
plt.plot(t, error_uldap, linestyle='--', dashes=(0.5,0.5), color='cyan', linewidth=2, label='ULDA+')

# configure and save plot
plt.legend(frameon=False)
plt.xlabel(r'$t$ (a.u.)', size=25)
plt.ylabel(r'$n_{\mathrm{error}}$  (a.u.)', size=25)
plt.tick_params(top='on', right='on')
plt.tick_params(direction='in')
plt.gcf().subplots_adjust(left=0.18)
plt.gcf().subplots_adjust(bottom=0.18)
plt.savefig('h2_td_error.pdf')
```

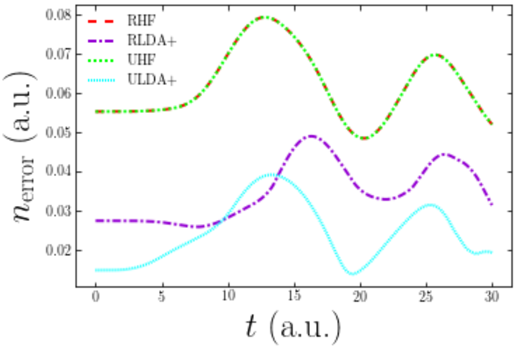


We will now plot the densities at the end of the simulation:

In [34]:

```
# plot densities
plt.plot(x, n_ext[-1,:], linestyle='-', dashes=(), color='k', linewidth=2, label='Exact')
plt.plot(x, n_rhf[-1,:], linestyle='--', dashes=(3, 3), color='red', linewidth=2, label='RHF')
plt.plot(x, n_rldap[-1,:], linestyle='--', dashes=(3,1,1,1), color='darkviolet', linewidth=2, label='RLDA+
plt.plot(x, n_uhf[-1,:], linestyle='--', dashes=(1, 1), color='lime', linewidth=2, label='UHF')
plt.plot(x, n_uldap[-1,:], linestyle='--', dashes=(0.5,0.5), color='cyan', linewidth=2, label='ULDA+')

# configure and save plot
plt.legend(frameon=False)
plt.xlabel(r'$x$ (a.u.)', size=25)
plt.ylabel(r'$n$ (a.u.)', size=25)
plt.tick_params(top='on', right='on')
plt.tick_params(direction='in')
plt.gcf().subplots_adjust(left=0.18)
plt.gcf().subplots_adjust(bottom=0.18)
plt.savefig('h2_td_den.pdf')
```

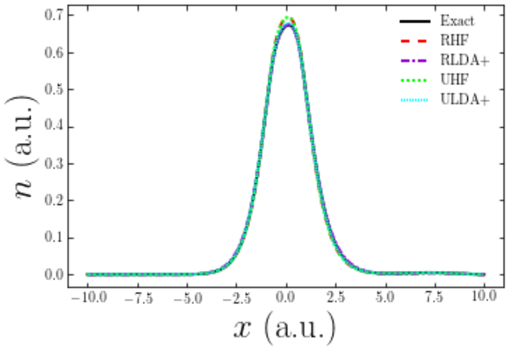


We will now plot the current densities at the end of the simulation:

In [35]:

```
# system the natural length
d = ds[E.argmin()]
i = E.argmin()

# import currents
I_ext = pickle.load(open('outputs/h2_{0}/raw/td_ext_cur.db'.format(i),'rb'))
I_uhf = pickle.load(open('outputs/h2_{0}/raw/td_uhf_cur.db'.format(i),'rb'))
I_rhf = pickle.load(open('outputs/h2_{0}/raw/td_rhf_cur.db'.format(i),'rb'))
I_uldap = pickle.load(open('outputs/h2_{0}/raw/td_uldap_cur.db'.format(i),'rb'))
I_rldap = pickle.load(open('outputs/h2_{0}/raw/td_rldap_cur.db'.format(i),'rb'))
```

In [36]:
```
# plot currents
plt.plot(x, I_ext[-1,:], linestyle='-', dashes=(), color='k', linewidth=2, label='Exact')
plt.plot(x, I_rhf[-1,:], linestyle='--', dashes=(3, 3), color='red', linewidth=2, label='RHF')
plt.plot(x, I_rldap[-1,:], linestyle='--', dashes=(3,1,1,1), color='darkviolet', linewidth=2, label='RLDA+
plt.plot(x, I_uhf[-1,:], linestyle='--', dashes=(1, 1), color='lime', linewidth=2, label='UHF')
plt.plot(x, I_uldap[-1,:], linestyle='--', dashes=(0.5,0.5), color='cyan', linewidth=2, label='ULDA+')

# configure and save plot
plt.legend(frameon=False)
plt.xlabel(r'$x$ (a.u.)', size=25)
plt.ylabel(r'$I$ (a.u.)', size=25)
plt.tick_params(top='on', right='on')
plt.tick_params(direction='in')
plt.gcf().subplots_adjust(left=0.18)
plt.gcf().subplots_adjust(bottom=0.18)
plt.savefig('h2_td_cur.pdf')
```

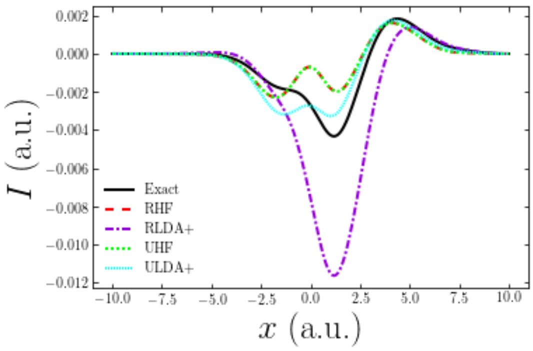


# 6. Time-dependence of charge density at stretched length due to external electric field

We will now apply a uniform electic field across our model hydrogen molecule (streched), and compare our approximxate methods to the exact real time evolving density:

In [37]:
```
# system the stretched length
d = ds[-1]
i = 59
print('i of stretched length = {0}'.format(i))
pm.space.v_ext = np.copy(v(x)) # set the external potential
pm.run.name = 'h2_{0}'.format(i)
pm.run.verbosity = 'default'

# set-up parameters for time dependence:
def vp(x):
    return -0.03*x # electric field of strength 0.08 a.u.
pm.sys.v_pert = vp
pm.setup_space()
pm.space.v_ext = np.copy(v(x)) # set the external potential
pm.run.time_dependence = True
pm.sys.tmax = 30.0 # Total real time
pm.sys.imax = 3001 # Number of real time iterations
```

```
i of stretched length = 59
```

In [38]:
```
# WARNING: Long Run! Does not need to be run again for rest of the script to work!
pm.hf.nu = 0.1
pm.ldap.nu = 0.1

# run the system with exact and approximate methods
pm.run.verbosity = 'default'
result_ext = iDEA.EXT2.main(pm)
result_uhf = iDEA.UHF.main(pm)
result_rhf = iDEA.RHF.main(pm)
result_uldap = iDEA.ULDAp.main(pm)
result_rldap = iDEA.RLDAp.main(pm)
```

In [39]:
```
# system the stretched length
d = ds[-1]
i = 59

# import densities
n_ext = pickle.load(open('outputs/h2_{0}/raw/td_ext_den.db'.format(i),'rb'))
n_uhf = pickle.load(open('outputs/h2_{0}/raw/td_uhf_den.db'.format(i),'rb'))
n_rhf = pickle.load(open('outputs/h2_{0}/raw/td_rhf_den.db'.format(i),'rb'))
n_uldap = pickle.load(open('outputs/h2_{0}/raw/td_uldap_den.db'.format(i),'rb'))
n_rldap = pickle.load(open('outputs/h2_{0}/raw/td_rldap_den.db'.format(i),'rb'))

# compute errors in the densities as a function of time
t = np.linspace(0.0, 30.0, 3001)
error_uhf = np.zeros(shape=pm.sys.imax)
error_rhf = np.zeros(shape=pm.sys.imax)
error_uldap = np.zeros(shape=pm.sys.imax)
error_rldap = np.zeros(shape=pm.sys.imax)
for i in range(pm.sys.imax):
    error_uhf[i] = np.sum(abs(n_ext[i,:] - n_uhf[i,:]))*dx
    error_rhf[i] = np.sum(abs(n_ext[i,:] - n_rhf[i,:]))*dx
    error_uldap[i] = np.sum(abs(n_ext[i,:] - n_uldap[i,:]))*dx
    error_rldap[i] = np.sum(abs(n_ext[i,:] - n_rldap[i,:]))*dx
```

In [40]:
```
# plot error curves
plt.plot(t, error_rhf, linestyle='--', dashes=(3, 3), color='red', linewidth=2, label='RHF')
plt.plot(t, error_rldap, linestyle='--', dashes=(3,1,1,1), color='darkviolet', linewidth=2, label='RLDA+')
plt.plot(t, error_uhf, linestyle='--', dashes=(1, 1), color='lime', linewidth=2, label='UHF')
plt.plot(t, error_uldap, linestyle='--', dashes=(0.5,0.5), color='cyan', linewidth=2, label='ULDA+')

# configure and save plot
plt.legend(frameon=False)
plt.xlabel(r'$t$ (a.u.)', size=25)
plt.ylabel(r'$n_{\mathrm{error}}$  (a.u.)', size=25)
plt.tick_params(top='on', right='on')
plt.tick_params(direction='in')
plt.gcf().subplots_adjust(left=0.18)
plt.gcf().subplots_adjust(bottom=0.18)
plt.savefig('h2_td_error_stretched.pdf')
```

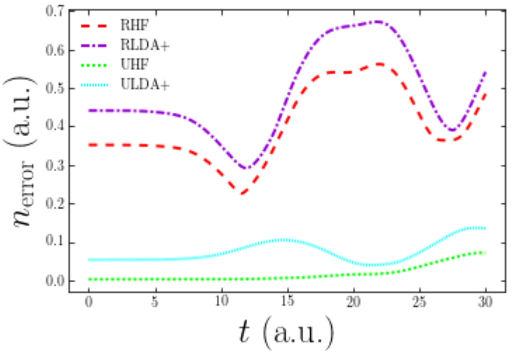


We will now plot the densities at the end of the simulation:

In [41]:
```
# plot densities
plt.plot(x, n_ext[-1,:], linestyle='-', dashes=(), color='k', linewidth=2, label='Exact')
plt.plot(x, n_rhf[-1,:], linestyle='--', dashes=(3, 3), color='red', linewidth=2, label='RHF')
plt.plot(x, n_rldap[-1,:], linestyle='--', dashes=(3,1,1,1), color='darkviolet', linewidth=2, label='RLDA+
plt.plot(x, n_uhf[-1,:], linestyle='--', dashes=(1, 1), color='lime', linewidth=2, label='UHF')
plt.plot(x, n_uldap[-1,:], linestyle='--', dashes=(0.5,0.5), color='cyan', linewidth=2, label='ULDA+')

# configure and save plot
plt.legend(frameon=False)
plt.xlabel(r'$x$ (a.u.)', size=25)
plt.ylabel(r'$n$ (a.u.)', size=25)
plt.tick_params(top='on', right='on')
plt.tick_params(direction='in')
plt.gcf().subplots_adjust(left=0.18)
plt.gcf().subplots_adjust(bottom=0.18)
plt.savefig('h2_td_den_stretched.pdf')
```

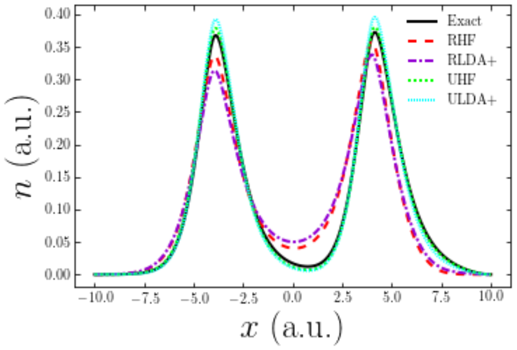


We will now plot the current densities at the end of the simulation:

In [42]:
```
# system the stretched length
i = 59

# import currents
I_ext = pickle.load(open('outputs/h2_{0}/raw/td_ext_cur.db'.format(i),'rb'))
I_uhf = pickle.load(open('outputs/h2_{0}/raw/td_uhf_cur.db'.format(i),'rb'))
I_rhf = pickle.load(open('outputs/h2_{0}/raw/td_rhf_cur.db'.format(i),'rb'))
I_uldap = pickle.load(open('outputs/h2_{0}/raw/td_uldap_cur.db'.format(i),'rb'))
I_rldap = pickle.load(open('outputs/h2_{0}/raw/td_rldap_cur.db'.format(i),'rb'))
```

In [43]:
```
# plot currents
plt.plot(x, I_ext[-1,:], linestyle='-', dashes=(), color='k', linewidth=2, label='Exact')
plt.plot(x, I_rhf[-1,:], linestyle='--', dashes=(3, 3), color='red', linewidth=2, label='RHF')
plt.plot(x, I_rldap[-1,:], linestyle='--', dashes=(3,1,1,1), color='darkviolet', linewidth=2, label='RLDA+
plt.plot(x, I_uhf[-1,:], linestyle='--', dashes=(1, 1), color='lime', linewidth=2, label='UHF')
plt.plot(x, I_uldap[-1,:], linestyle='--', dashes=(0.5,0.5), color='cyan', linewidth=2, label='ULDA+')

# configure and save plot
plt.legend(frameon=False)
plt.xlabel(r'$x$ (a.u.)', size=25)
plt.ylabel(r'$I$ (a.u.)', size=25)
plt.tick_params(top='on', right='on')
plt.tick_params(direction='in')
plt.gcf().subplots_adjust(left=0.18)
plt.gcf().subplots_adjust(bottom=0.18)
plt.savefig('h2_td_cur_stretched.pdf')
```

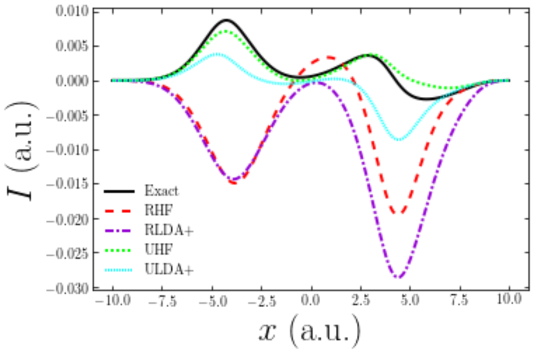


# 7. Features of the exact $V_c$

We will now look at the exact Vc and both RHFKS and UHFKS at the natural lenght, and fully stretched length:

In [44]:
```
import iDEA.RHFKS
import iDEA.UHFKS
```

In [45]:
```
# WARNING: Long Run! Does not need to be run again for rest of the script to work!

# first at the natural length
d = ds[E.argmin()]
i = E.argmin()
pm.run.time_dependence = False
pm.space.v_ext = np.copy(v(x)) # set the external potential
pm.run.name = 'h2_{0}'.format(i)
result_rhfks = iDEA.RHFKS.main(pm, 'ext')
result_uhfks = iDEA.UHFKS.main(pm, 'ext')
```

In [46]:
```
i = E.argmin()
vc_rhfks_natural = pickle.load(open('outputs/h2_{0}/raw/gs_extrhfks_vc.db'.format(i),'rb'))
vc_uhfks_natural = pickle.load(open('outputs/h2_{0}/raw/gs_extuhfks_vc.db'.format(i),'rb'))

# plot energy curve
plt.plot(x, vc_uhfks_natural+0.027, linestyle='-', color='lime', linewidth=2, label='UHFKS')
plt.plot(x, vc_rhfks_natural-0.005, linestyle=':', color='red', linewidth=2, label='RHFKS')

# configure and save plot
plt.legend(frameon=False)
plt.xlabel(r'$x$ (a.u.)', size=25)
plt.ylabel(r'$V_{\mathrm{c}}$ (a.u.)', size=25)
plt.tick_params(top='on', right='on')
plt.tick_params(direction='in')
plt.gcf().subplots_adjust(left=0.18)
plt.gcf().subplots_adjust(bottom=0.18)
plt.savefig('exact_vc_natural.pdf')
```

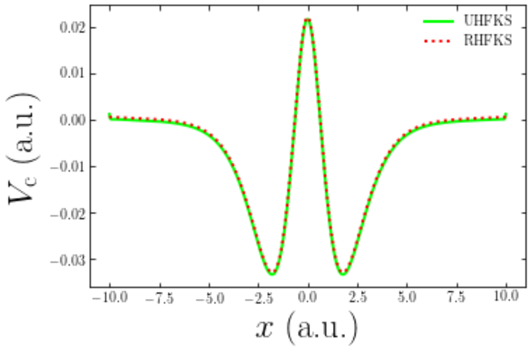


In [47]:
```
# WARNING: Long Run! Does not need to be run again for rest of the script to work!

# then at the stretched length
d = ds[44]
i = 44
pm.run.time_dependence = False
pm.space.v_ext = np.copy(v(x)) # set the external potential
pm.run.name = 'h2_{0}'.format(i)
pm.hfks.mu = 0.01 # stability parameters
pm.hfks.p = 0.05  # stability parameters
pm.hf.nu = 0.1    # stability parameters
result_rhfks = iDEA.RHFKS.main(pm, 'ext')
result_uhfks = iDEA.UHFKS.main(pm, 'ext')
```

In [48]:
```
i = 44
vc_rhfks_stretched = pickle.load(open('outputs/h2_{0}/raw/gs_extrhfks_vc.db'.format(i),'rb'))
vc_uhfks_stretched = pickle.load(open('outputs/h2_{0}/raw/gs_extuhfks_vc.db'.format(i),'rb'))

# plot energy curve
plt.plot(x, vc_rhfks_stretched-0.2, linestyle=':', color='lime', linewidth=2, label='RHFKS')
plt.plot(x, vc_uhfks_stretched+0.04, linestyle='-', color='red', linewidth=2, label='UHFKS')

# configure and save plot
plt.legend(frameon=False)
plt.xlabel(r'$x$ (a.u.)', size=25)
plt.ylabel(r'$V_{\mathrm{c}}$ (a.u.)', size=25)
plt.tick_params(top='on', right='on')
plt.tick_params(direction='in')
plt.gcf().subplots_adjust(left=0.18)
plt.gcf().subplots_adjust(bottom=0.18)
plt.savefig('exact_vc_stretched.pdf')
```

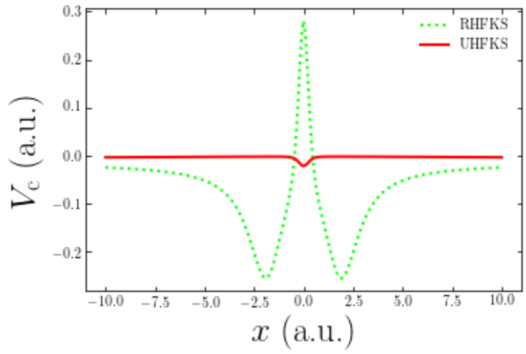

Supplement: Supplementary file 1 [file results.pdf]
