# Supplementary material for: Accurate real-time evolution of electron densities and ground-state properties from generalized Kohn-Sham theory
Source: arXiv:1909.02510 source file (2020-01-11)

```
In [1]: %matplotlib inline
import warnings
warnings.filterwarnings('ignore')
#import matplotlib
#matplotlib.use('Agg')
```

# 1. Designing the model molecule

## 1.1. Determining the softening parameters for H atoms in iDEA

In order to closely approach a real  $H_2$  molecule in iDEA we need to use appropriate softening parameters. There are two such parameters, one for the electrons ( $\alpha$ )

$$V_e(x) = \frac{1}{|x| + \alpha},$$

and one for the protons ( $\beta$ )

$$V_p(x) = \frac{1}{|x| + \beta}.$$

As shown in [M.J.P Hodgson's thesis \(https://www.researchgate.net/publication/333760017\\_Electrons\\_in\\_model\\_nanostructures\)](https://www.researchgate.net/publication/333760017_Electrons_in_model_nanostructures) (Appendix A.2) to model as closely as possible the interaction of two charged disks the appropriate electron softening parameter is:

$$\alpha = 1.0$$

Now we will determine the value of  $\beta$ . To determine it we will compute the total energy of a one-electron atom with the following external potential:

$$V_{\text{ext}}(x) = \frac{1}{|x| + \beta}.$$

As we want to converge the scale of  $\beta$  will write it as:

$$V_{\text{ext}}(x) = \frac{1}{|x| + 10^{-b}}.$$

And then plot  $E(b)$  to see what value of  $b$  gives the correct value of the ground-state energy  $E = -13.6\text{eV}$ .

This in  $E = -0.5$  (a.u) in atomic units.

```
In [2]: E_target = -0.5
```

First lets just try  $b = 0$ :

```
In [3]: # import all needed modules
import numpy as np
import scipy as sp
import matplotlib.pyplot as plt
plt.rc('text', usetex=True) # use LaTeX
from iDEA.input import Input
```

```
In [4]: # set up the system
pm = Input()
pm.sys.NE = 1 # number of electrons
pm.sys.grid = 1001 # number of grid points
pm.sys.xmax = 10.0 # lenght of system L = 2*xmax
pm.sys.acon = 1.0 # the value of alpha
pm.run.name = 'h_atom'

b = 0
def v(x):
    return -1.0/(abs(x)+10**-b) # the value of beta=10^-b

pm.setup_space()
pm.run.setup_space = False
pm.space.v_ext = np.copy(v(pm.space.grid)) # set the external potential
```

In [5]: `# use EXT1 to find exact energy`

```
import iDEA.EXT1
pm.make_dirs()
pm.check()
result = iDEA.EXT1.main(pm)
```

EXT: constructing arrays

EXT: solving the time-independent Schrodinger equation

EXT: calculated the ground-state

E0 = -0.50003

We can plot the external potential and ground-state charge density:

In [6]: `# plot  $n$  and  $V_{\text{ext}}$  for  $b=0$`

```
x = pm.space.grid
plt.plot(x, result.gs_ext_den, linewidth=2, linestyle='-', color='k', label='$n$')
plt.plot(x, result.gs_ext_vxt, linewidth=2, linestyle='--', color='b', label='$V_{\mathrm{ext}}$')

# configure and save plot
plt.legend(frameon=False)
plt.xlabel(r'$x$ (a.u.)', size=25)
plt.ylabel(r'$n$, $V_{\mathrm{ext}}$ (a.u.)', size=25)
plt.tick_params(top='on', right='on')
plt.tick_params(direction='in')
plt.gcf().subplots_adjust(left=0.18)
plt.gcf().subplots_adjust(bottom=0.18)
plt.savefig('h_atom.pdf')
```

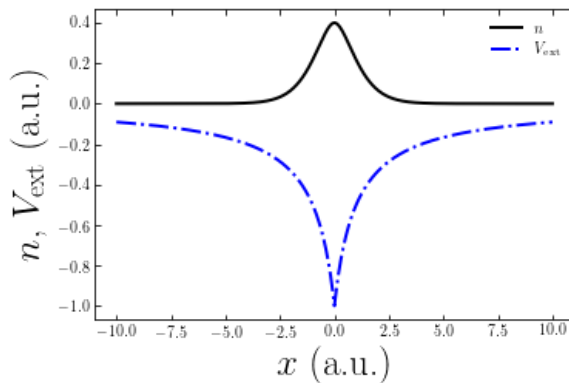

So this value already gives a remarkably close energy to the target energy with an absolute error of:

In [7]: `E_error = abs(E_target - result.gs_ext_E)
print('E_error = {} a.u.'.format(E_error))`

E\_error = 2.649331702464508e-05 a.u.

To make sure this isn't a fluke let's loop over  $b$  to find the best  $b$ :

In [8]: `pm.run.verbosity = 'low'
b_list = [0.0, 1.0, 2.0, 3.0, 4.0, 5.0, 6.0]
E_list = []
error_list = []
for i in range(0, len(b_list)):
 b = b_list[i]
 pm.space.v_ext = np.copy(v(pm.space.grid)) # set the external potential
 result = iDEA.EXT1.main(pm)
 E_list.append(result.gs_ext_E)
 error_list.append(abs(E_target - result.gs_ext_E))
 print('b = {0}, E = {1}, error = {2}'.format(b_list[i], E_list[i], error_list[i]))`

```
b = 0.0, E = -0.5000264933170246, error = 2.649331702464508e-05
b = 1.0, E = -2.7312164568047055, error = 2.2312164568047055
b = 2.0, E = -12.371601413502413, error = 11.871601413502413
b = 3.0, E = -196.0966496559432, error = 195.5966496559432
b = 4.0, E = -7099.571324878994, error = 7099.071324878994
b = 5.0, E = -96364.72964351632, error = 96364.22964351632
b = 6.0, E = -996280.9352739786, error = 996280.4352739786
```

So we know the value of  $\beta$  is about  $10^0 = 1.0$  let's now search in the region of 1 (from 0.5 to 1.5):

```
In [9]: def v(x):
        return -1.0/(abs(x)+beta) # the value of beta

pm.run.verbosity = 'low'
beta_list = [0.5, 0.6, 0.7, 0.8, 0.9, 1.0, 1.1, 1.2, 1.3, 1.4, 1.5]
E_list = []
error_list = []
for i in range(0, len(beta_list)):
    beta = beta_list[i]
    pm.space.v_ext = np.copy(v(pm.space.grid)) # set the external potential
    result = iDEA.EXT1.main(pm)
    E_list.append(result.gs_ext_E)
    error_list.append(abs(E_target - result.gs_ext_E))
    print('beta = {0}, E = {1}, error = {2}'.format(beta_list[i], E_list[i], error_list[i]))

beta = 0.5, E = -0.8599751320146161, error = 0.35997513201461606
beta = 0.6, E = -0.7474941859982969, error = 0.24749418599829687
beta = 0.7, E = -0.6630304287461015, error = 0.16303042874610152
beta = 0.8, E = -0.5970182718805466, error = 0.09701827188054657
beta = 0.9, E = -0.5438550104249282, error = 0.04385501042492823
beta = 1.0, E = -0.5000264933170246, error = 2.649331702464508e-05
beta = 1.1, E = -0.4632095864741271, error = 0.03679041352587292
beta = 1.2, E = -0.43180310437046776, error = 0.06819689562953224
beta = 1.3, E = -0.40466535814986365, error = 0.09533464185013635
beta = 1.4, E = -0.3809590292771655, error = 0.11904097072283448
beta = 1.5, E = -0.36005524621527774, error = 0.13994475378472226
```

Plotting the error in  $E$  against  $\beta$ :

```
In [10]: # plot E vs beta
plt.plot(beta_list, error_list, linewidth=2, linestyle='--', color='k')

# configure and save plot
plt.xlabel(r'$\beta$ (a.u.)', size=25)
plt.ylabel(r'$E_{\mathrm{error}}$ (a.u.)', size=25)
plt.tick_params(top='on', right='on')
plt.tick_params(direction='in')
plt.gcf().subplots_adjust(left=0.18)
plt.gcf().subplots_adjust(bottom=0.18)
plt.savefig('softening.pdf')
```

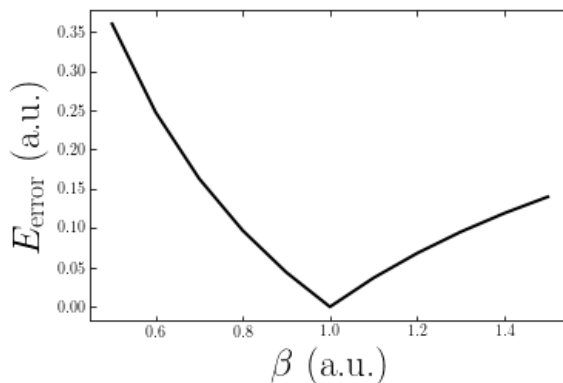

So the final values are:  $\alpha = 1.0$  and  $\beta = 1.0$ , in iDEA these give the value of the energy of our model hydrogen atom to be:  $E = -13.6\text{eV}$ .

## 1.2 Testing our model molecule

Here we will investigate a model molecule to see if a covalent bond forms between a system of two opposite-spin electron system comprised of two proton wells separated by a distance  $d$ . We will plot the total energy  $E = E_e + E_p$  against distance  $d$ .

We will calculate  $E(d)$  for our system to determine the bond length:

```
In [11]: # set up the system
pm = Input()
pm.run.name = 'h2_test'
pm.sys.NE = 2 # number of electrons
pm.sys.spin = 'opposite' # both electrons treated as opposite spin
pm.sys.grid = 501
pm.sys.xmax = 10.0
pm.sys.acon = 1.0 # value of alpha (see section 1.1)
beta = 1.0 # value of beta (see section 1.1)
pm.setup_space()
pm.run.setup_space = False
```

To make sure the system is wide enough let's plot the external potential at the maximum width (8.0 a.u):

```
In [12]: d = 8.0
def v(x):
    return -3.0/(0.8*abs(x-0.5*d)+2)-1.0/(abs(x+0.5*d)+1)
x = np.linspace(-pm.sys.xmax, pm.sys.xmax, pm.sys.grid)
dx = x[1] - x[0]
plt.plot(x, v(x), linestyle='-', color='k')

# configure and save plot
plt.xlabel(r'$x$ (a.u.)', size=25)
plt.ylabel(r'$V_{\mathrm{ext}}$ (a.u.)', size=25)
plt.tick_params(top='on', right='on')
plt.tick_params(direction='in')
plt.gcf().subplots_adjust(left=0.18)
plt.gcf().subplots_adjust(bottom=0.18)
plt.savefig('v.pdf')
```

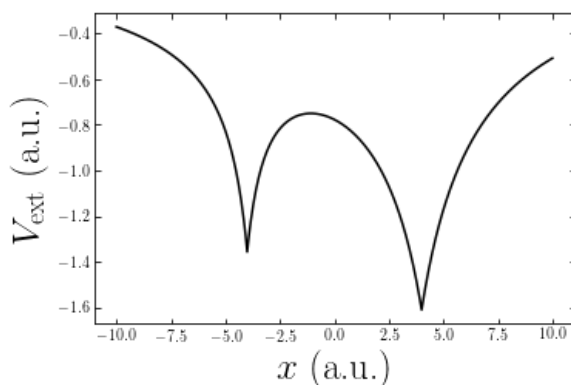

```
In [13]: # make array of distances
ds = np.linspace(0.0, 8.0, 60)
```

```
In [14]: # WARNING: Long Run! Does not need to be run again for rest of the script to work!

# main loop, stretching the molecule from 0 to 8 a.u
for i in range(ds.shape[0]):
    d = ds[i]
    print('running d={0}'.format(d))
    pm.run.name = 'h2_{0}'.format(i)
    pm.space.v_ext = np.copy(v(x)) # set the external potential
    pm.make_dirs()
    pm.run.verbosity = 'low'
    result = iDEA.EXT2.main(pm)
```

```
In [15]: # load in energies and distances
E_list = []
for i in range(ds.shape[0]):
    E = pickle.load(open('outputs/h2_{0}/raw/gs_ext_E.db'.format(i), 'rb'))
    E_list.append(E)

# convert to numpy arrays
E_e = np.array(E_list)

# add in proton energy
E_p = 1.0/(np.abs(ds)+beta)
E = E_e + E_p
```

```
In [16]: # plot energy curve
plt.plot(ds, E, linestyle='--', color='k', linewidth=2)

# configure and save plot
plt.xlabel(r'$d$ (a.u.)', size=25)
plt.ylabel(r'$E$ (a.u.)', size=25)
plt.tick_params(top='on', right='on')
plt.tick_params(direction='in')
plt.gcf().subplots_adjust(left=0.18)
plt.gcf().subplots_adjust(bottom=0.18)
plt.savefig('exact_h2.pdf')
```

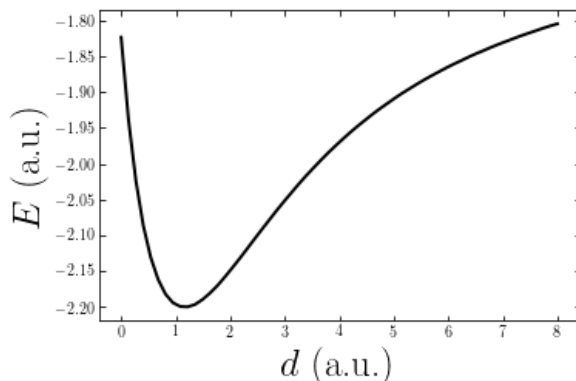

## 2. Exact and approximate energy dissociation curves

We will now compare each of our approximate methods (RHF, RDA+, UHF, ULDA+) against the exact dissociation curves for our model hydrogen molecule:

```
In [17]: # imports iDEA modules
import iDEA.RHF
import iDEA.UHF
import iDEA.RLDap
import iDEA.ULDAp

# allow HF and LDA+ methods to converge for large stretched limit
pm.hf.con = 1e-10
pm.ldap.con = 1e-10
```

```
In [18]: # WARNING: Long Run! Does not need to be run again for rest of the script to work!

# main loop, stretching the molecule from 0 to 8 a.u
for i in range(ds.shape[0]):
    d = ds[i]
    print('running d={0}'.format(d))
    pm.run.name = 'h2_{0}'.format(i)
    pm.space.v_ext = np.copy(v(x)) # set the external potential
    if i > 44: # change the mixing parameter for the large distances for stability
        pm.hf.nu = 0.1
        pm.ldap.nu = 0.1
    result_rhf = iDEA.RHF.main(pm)
    result_uhf = iDEA.UHF.main(pm)
    result_rldap = iDEA.RLDap.main(pm)
    result_uldap = iDEA.ULDAp.main(pm)
```

```
In [19]: # load in energies and distances
E_rhf = []
E_uhf = []
E_rldap = []
E_uldap = []
for i in range(ds.shape[0]):
    E0 = pickle.load(open('outputs/h2_{0}/raw/gs_rhf_E.db'.format(i), 'rb'))
    E_rhf.append(E0)
    E0 = pickle.load(open('outputs/h2_{0}/raw/gs_uhf_E.db'.format(i), 'rb'))
    E_uhf.append(E0)
    E0 = pickle.load(open('outputs/h2_{0}/raw/gs_rldap_E.db'.format(i), 'rb'))
    E_rldap.append(E0)
    E0 = pickle.load(open('outputs/h2_{0}/raw/gs_uldap_E.db'.format(i), 'rb'))
    E_uldap.append(E0)

# convert to numpy arrays
E_rhf = np.array(E_rhf)
E_uhf = np.array(E_uhf)
E_rldap = np.array(E_rldap)
E_uldap = np.array(E_uldap)

# add in proton energy
E_p = 1.0/(np.abs(ds)+beta)
E_rhf += E_p
E_uhf += E_p
E_rldap += E_p
E_uldap += E_p
```

```
In [20]: # plot energy curve
plt.plot(ds, E, linestyle='-', dashes=(), color='k', linewidth=2, label='Exact')
plt.plot(ds, E_rhf, linestyle='--', dashes=(3, 3), color='red', linewidth=2, label='RHF')
plt.plot(ds, E_uhf, linestyle='--', dashes=(1, 1), color='lime', linewidth=2, label='UHF')
plt.plot(ds, E_rldap, linestyle='--', dashes=(3,1,1,1), color='darkviolet', linewidth=2, label='RLDA+')
plt.plot(ds, E_uldap, linestyle='--', dashes=(0.5,0.5), color='cyan', linewidth=2, label='ULDA+')

# configure and save plot
plt.legend(frameon=False)
plt.xlabel(r'$d$ (a.u.)', size=25)
plt.ylabel(r'$E$ (a.u.)', size=25)
plt.tick_params(top='on', right='on')
plt.tick_params(direction='in')
plt.gcf().subplots_adjust(left=0.18)
plt.gcf().subplots_adjust(bottom=0.18)
plt.savefig('h2.pdf')
```

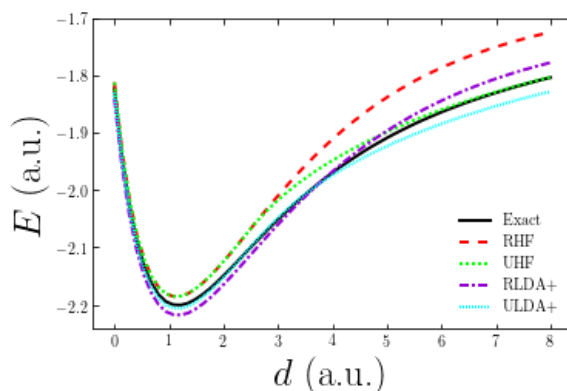

### 3. Charge density at natural length

We will now compare the accuracy of the charge density of each of the approximate methods at the molecules natural length:

```
In [21]: # system the natural length
d = ds[E.argmin()]
i = E.argmin()
pm.space.v_ext = np.copy(v(x)) # set the external potential

# load in the densities
n = pickle.load(open('outputs/h2_{0}/raw/gs_ext_den.db'.format(i), 'rb'))
n_rhf = pickle.load(open('outputs/h2_{0}/raw/gs_rhf_den.db'.format(i), 'rb'))
n_uhf = pickle.load(open('outputs/h2_{0}/raw/gs_uhf_den.db'.format(i), 'rb'))
n_rldap = pickle.load(open('outputs/h2_{0}/raw/gs_rldap_den.db'.format(i), 'rb'))
n_uldap = pickle.load(open('outputs/h2_{0}/raw/gs_uldap_den.db'.format(i), 'rb'))
```

```
In [22]: # plot densities
plt.plot(x, n, linestyle='-', dashes=(), color='k', linewidth=2, label='Exact')
plt.plot(x, n_rhf, linestyle='--', dashes=(3, 3), color='red', linewidth=2, label='RHF')
plt.plot(x, n_rldap, linestyle='--', dashes=(3,1,1,1), color='darkviolet', linewidth=2, label='R')
plt.plot(x, n_uhf, linestyle='--', dashes=(1, 1), color='lime', linewidth=2, label='UHF')
plt.plot(x, n_uldap, linestyle='--', dashes=(0.5,0.5), color='cyan', linewidth=2, label='ULDA+')

# configure and save plot
plt.legend(frameon=False)
plt.xlabel(r'$x$ (a.u.)', size=25)
plt.ylabel(r'$n$ (a.u.)', size=25)
plt.tick_params(top='on', right='on')
plt.tick_params(direction='in')
plt.gcf().subplots_adjust(left=0.18)
plt.gcf().subplots_adjust(bottom=0.18)
plt.savefig('h2_natural.pdf')
```

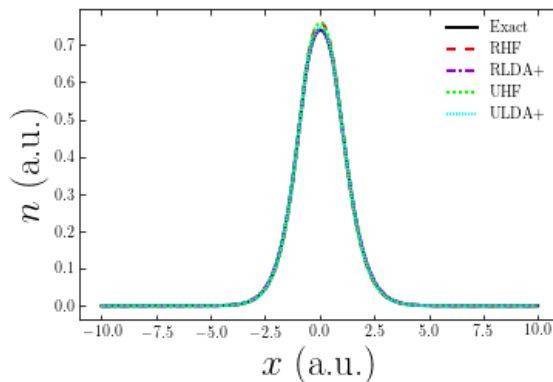

## 4. Charge density at stretched (dissociated) length

We will now compare the accuracy of the charge density of each of the approximate methods at the molecules stretched (dissociated) length:

```
In [23]: # system the stretched length
d = ds[-1]
i = 59
pm.space.v_ext = np.copy(v(x)) # set the external potential

# load in the densities
n = pickle.load(open('outputs/h2_{0}/raw/gs_ext_den.db'.format(i), 'rb'))
n_rhf = pickle.load(open('outputs/h2_{0}/raw/gs_rhf_den.db'.format(i), 'rb'))
n_uhf = pickle.load(open('outputs/h2_{0}/raw/gs_uhf_den.db'.format(i), 'rb'))
n_rldap = pickle.load(open('outputs/h2_{0}/raw/gs_rldap_den.db'.format(i), 'rb'))
n_uldap = pickle.load(open('outputs/h2_{0}/raw/gs_uldap_den.db'.format(i), 'rb'))
```

```
In [24]: # plot densities
plt.plot(x, n, linestyle='-', dashes=(), color='k', linewidth=2, label='Exact')
plt.plot(x, n_rhf, linestyle='--', dashes=(3, 3), color='red', linewidth=2, label='RHF')
plt.plot(x, n_rldap, linestyle='--', dashes=(3,1,1,1), color='darkviolet', linewidth=2, label='R')
plt.plot(x, n_uhf, linestyle='--', dashes=(1, 1), color='lime', linewidth=2, label='UHF')
plt.plot(x, n_uldap, linestyle='--', dashes=(0.5,0.5), color='cyan', linewidth=2, label='ULDA+')

# configure and save plot
plt.legend(frameon=False)
plt.xlabel(r'$x$ (a.u.)', size=25)
plt.ylabel(r'$n$ (a.u.)', size=25)
plt.tick_params(top='on', right='on')
plt.tick_params(direction='in')
plt.gcf().subplots_adjust(left=0.18)
plt.gcf().subplots_adjust(bottom=0.18)
plt.savefig('h2_stretched.pdf')
```

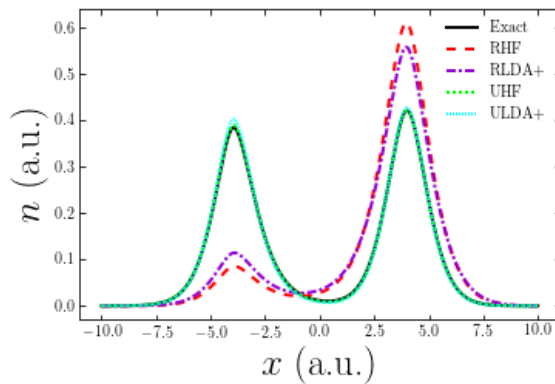

## 5. Time-dependence of charge density at natural length due to external electric field

We will now apply a uniform electric field across our model hydrogen molecule, and compare our approximate methods to the exact real time evolving density:

```
In [25]: # system the natural length
d = ds[E.argmax()]
i = E.argmax()
print('i of natural length = {}'.format(i))
pm.space.v_ext = np.copy(v(x)) # set the external potential
pm.run.name = 'h2_{}'.format(i)
pm.run.verbosity = 'default'

# set-up parameters for time dependence:
def vp(x):
    return -0.03*x # electric field of strength 0.08 a.u.
pm.sys.v_pert = vp
pm.setup_space()
pm.space.v_ext = np.copy(v(x)) # set the external potential
pm.run.time_dependence = True
pm.sys.tmax = 30.0 # Total real time
pm.sys.imax = 3001 # Number of real time iterations

i of natural length = 9
```

```
In [26]: # WARNING: Long Run! Does not need to be run again for rest of the script to work!

# run the system with exact and approximate methods
pm.run.verbosity = 'default'
result_ext = iDEA.EXT2.main(pm)
result_uhf = iDEA.UHF.main(pm)
result_rhf = iDEA.RHF.main(pm)
result_uldap = iDEA.ULDAp.main(pm)
result_rldap = iDEA.RLDAp.main(pm)
```



```
In [27]: # import densities
n_ext = pickle.load(open('outputs/h2_{0}/raw/td_ext_den.db'.format(i), 'rb'))
n_uhf = pickle.load(open('outputs/h2_{0}/raw/td_uhf_den.db'.format(i), 'rb'))
n_rhf = pickle.load(open('outputs/h2_{0}/raw/td_rhf_den.db'.format(i), 'rb'))
n_uldap = pickle.load(open('outputs/h2_{0}/raw/td_uldap_den.db'.format(i), 'rb'))
n_rldap = pickle.load(open('outputs/h2_{0}/raw/td_rldap_den.db'.format(i), 'rb'))

# compute errors in the densities as a function of time
t = np.linspace(0.0, 30.0, 3001)
error_uhf = np.zeros(shape=pm.sys.imax)
error_rhf = np.zeros(shape=pm.sys.imax)
error_uldap = np.zeros(shape=pm.sys.imax)
error_rldap = np.zeros(shape=pm.sys.imax)
for i in range(pm.sys.imax):
    error_uhf[i] = np.sum(abs(n_ext[i,:] - n_uhf[i,:]))*dx
    error_rhf[i] = np.sum(abs(n_ext[i,:] - n_rhf[i,:]))*dx
    error_uldap[i] = np.sum(abs(n_ext[i,:] - n_uldap[i,:]))*dx
    error_rldap[i] = np.sum(abs(n_ext[i,:] - n_rldap[i,:]))*dx

In [28]: # plot error curves
plt.plot(t, error_rhf, linestyle='--', dashes=(3, 3), color='red', linewidth=2, label='RHF')
plt.plot(t, error_rldap, linestyle='--', dashes=(3,1,1,1), color='darkviolet', linewidth=2, label='RLDA+')
plt.plot(t, error_uhf, linestyle='--', dashes=(1, 1), color='lime', linewidth=2, label='UHF')
plt.plot(t, error_uldap, linestyle='--', dashes=(0.5,0.5), color='cyan', linewidth=2, label='ULD')

# configure and save plot
plt.legend(frameon=False)
plt.xlabel(r'$t$ (a.u.)', size=25)
plt.ylabel(r'$n_{\mathrm{error}}$ (a.u.)', size=25)
plt.tick_params(top='on', right='on')
plt.tick_params(direction='in')
plt.gcf().subplots_adjust(left=0.18)
plt.gcf().subplots_adjust(bottom=0.18)
plt.savefig('h2_td_error.pdf')
```

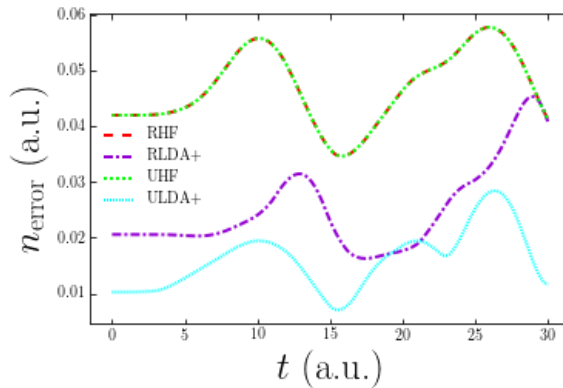

We will now plot the densities at the end of the simulation:

```
In [29]: # plot densities
plt.plot(x, n_ext[-1,:], linestyle='-', dashes=(), color='k', linewidth=2, label='Exact')
plt.plot(x, n_rhf[-1,:], linestyle='--', dashes=(3, 3), color='red', linewidth=2, label='RHF')
plt.plot(x, n_rldap[-1,:], linestyle='--', dashes=(3,1,1,1), color='darkviolet', linewidth=2, label='RLDA+')
plt.plot(x, n_uhf[-1,:], linestyle='--', dashes=(1, 1), color='lime', linewidth=2, label='UHF')
plt.plot(x, n_uldap[-1,:], linestyle='--', dashes=(0.5,0.5), color='cyan', linewidth=2, label='ULDA+')

# configure and save plot
plt.legend(frameon=False)
plt.xlabel(r'$x$ (a.u.)', size=25)
plt.ylabel(r'$n$ (a.u.)', size=25)
plt.tick_params(top='on', right='on')
plt.tick_params(direction='in')
plt.gcf().subplots_adjust(left=0.18)
plt.gcf().subplots_adjust(bottom=0.18)
plt.savefig('h2_td_den.pdf')
```

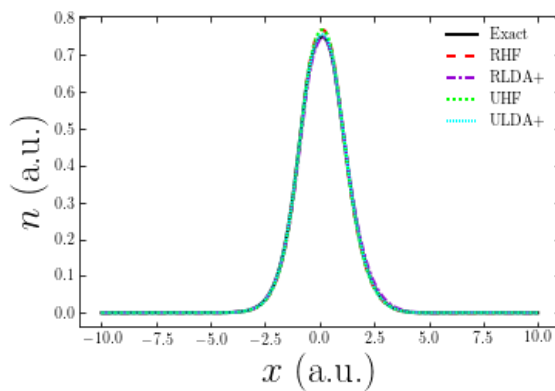

We will now plot the current densities at the end of the simulation:

```
In [30]: # system the natural length
d = ds[E.argmax()]
i = E.argmax()

# import currents
I_ext = pickle.load(open('outputs/h2_{0}/raw/td_ext_cur.db'.format(i), 'rb'))
I_uhf = pickle.load(open('outputs/h2_{0}/raw/td_uhf_cur.db'.format(i), 'rb'))
I_rhf = pickle.load(open('outputs/h2_{0}/raw/td_rhf_cur.db'.format(i), 'rb'))
I_uldap = pickle.load(open('outputs/h2_{0}/raw/td_uldap_cur.db'.format(i), 'rb'))
I_rldap = pickle.load(open('outputs/h2_{0}/raw/td_rldap_cur.db'.format(i), 'rb'))
```

```
In [31]: # plot currents
plt.plot(x, I_ext[-1,:], linestyle='-', dashes=(), color='k', linewidth=2, label='Exact')
plt.plot(x, I_rhf[-1,:], linestyle='--', dashes=(3, 3), color='red', linewidth=2, label='RHF')
plt.plot(x, I_rldap[-1,:], linestyle='--', dashes=(3,1,1,1), color='darkviolet', linewidth=2, label='RLDA+')
plt.plot(x, I_uhf[-1,:], linestyle='--', dashes=(1, 1), color='lime', linewidth=2, label='UHF')
plt.plot(x, I_uldap[-1,:], linestyle='--', dashes=(0.5,0.5), color='cyan', linewidth=2, label='ULDA+')

# configure and save plot
plt.legend(frameon=False)
plt.xlabel(r'$x$ (a.u.)', size=25)
plt.ylabel(r'$I$ (a.u.)', size=25)
plt.tick_params(top='on', right='on')
plt.tick_params(direction='in')
plt.gcf().subplots_adjust(left=0.18)
plt.gcf().subplots_adjust(bottom=0.18)
plt.savefig('h2_td_cur.pdf')
```

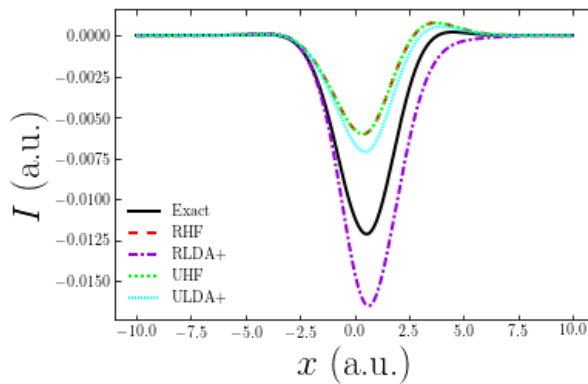

## 6. Time-dependence of charge density at stretched length due to external electric field

We will now apply a uniform electric field across our model hydrogen molecule (stretched), and compare our approximate methods to the exact real time evolving density:

```
In [32]: # system the stretched length
d = ds[59]
i = 59
print('i of stretched length = {0}'.format(i))
pm.space.v_ext = np.copy(v(x)) # set the external potential
pm.run.name = 'h2_{0}'.format(i)
pm.run.verbosity = 'default'

# set-up parameters for time dependence:
def vp(x):
    return -0.03*x # electric field of strength 0.08 a.u.
pm.sys.v_pert = vp
pm.setup_space()
pm.space.v_ext = np.copy(v(x)) # set the external potential
pm.run.time_dependence = True
pm.sys.tmax = 30.0 # Total real time
pm.sys.imax = 3001 # Number of real time iterations

i of stretched length = 59
```

```
In [33]: # WARNING: Long Run! Does not need to be run again for rest of the script to work!

# run the system with exact and approximate methods
pm.run.verbosity = 'default'
result_ext = iDEA.EXT2.main(pm)
result_uhf = iDEA.UHF.main(pm)
result_rhf = iDEA.RHF.main(pm)
result_uldap = iDEA.ULDAp.main(pm)
result_rldap = iDEA.RLDAp.main(pm)
```

```
In [34]: # import densities
n_ext = pickle.load(open('outputs/h2_{0}/raw/td_ext_den.db'.format(i), 'rb'))
n_uhf = pickle.load(open('outputs/h2_{0}/raw/td_uhf_den.db'.format(i), 'rb'))
n_rhf = pickle.load(open('outputs/h2_{0}/raw/td_rhf_den.db'.format(i), 'rb'))
n_uldap = pickle.load(open('outputs/h2_{0}/raw/td_uldap_den.db'.format(i), 'rb'))
n_rldap = pickle.load(open('outputs/h2_{0}/raw/td_rldap_den.db'.format(i), 'rb'))

# compute errors in the densities as a function of time
t = np.linspace(0.0, 30.0, 3001)
error_uhf = np.zeros(shape=pm.sys.imax)
error_rhf = np.zeros(shape=pm.sys.imax)
error_uldap = np.zeros(shape=pm.sys.imax)
error_rldap = np.zeros(shape=pm.sys.imax)
for i in range(pm.sys.imax):
    error_uhf[i] = np.sum(abs(n_ext[i,:] - n_uhf[i,:]))*dx
    error_rhf[i] = np.sum(abs(n_ext[i,:] - n_rhf[i,:]))*dx
    error_uldap[i] = np.sum(abs(n_ext[i,:] - n_uldap[i,:]))*dx
    error_rldap[i] = np.sum(abs(n_ext[i,:] - n_rldap[i,:]))*dx

In [35]: # plot error curves
plt.plot(t, error_rhf, linestyle='--', dashes=(3, 3), color='red', linewidth=2, label='RHF')
plt.plot(t, error_rldap, linestyle='--', dashes=(3,1,1,1), color='darkviolet', linewidth=2, label='RLDA+')
plt.plot(t, error_uhf, linestyle='--', dashes=(1, 1), color='lime', linewidth=2, label='UHF')
plt.plot(t, error_uldap, linestyle='--', dashes=(0.5,0.5), color='cyan', linewidth=2, label='ULD')

# configure and save plot
plt.legend(frameon=False)
plt.xlabel(r'$t$ (a.u.)', size=25)
plt.ylabel(r'$n_{\mathrm{error}}$ (a.u.)', size=25)
plt.tick_params(top='on', right='on')
plt.tick_params(direction='in')
plt.gcf().subplots_adjust(left=0.18)
plt.gcf().subplots_adjust(bottom=0.18)
plt.savefig('h2_td_error_stretched.pdf')
```

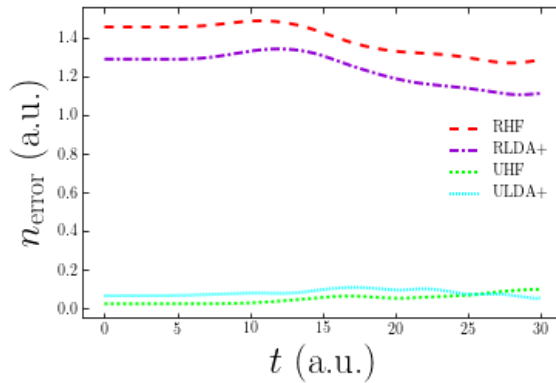

We will now plot the densities at the end of the simulation:

```
In [36]: # plot densities
plt.plot(x, n_ext[-1,:], linestyle='-', dashes=(), color='k', linewidth=2, label='Exact')
plt.plot(x, n_rhf[-1,:], linestyle='--', dashes=(3, 3), color='red', linewidth=2, label='RHF')
plt.plot(x, n_rldap[-1,:], linestyle='--', dashes=(3,1,1,1), color='darkviolet', linewidth=2, label='RLDA+')
plt.plot(x, n_uhf[-1,:], linestyle='--', dashes=(1, 1), color='lime', linewidth=2, label='UHF')
plt.plot(x, n_uldap[-1,:], linestyle='--', dashes=(0.5,0.5), color='cyan', linewidth=2, label='ULD+')

# configure and save plot
plt.legend(frameon=False)
plt.xlabel(r'$x$ (a.u.)', size=25)
plt.ylabel(r'$n$ (a.u.)', size=25)
plt.tick_params(top='on', right='on')
plt.tick_params(direction='in')
plt.gcf().subplots_adjust(left=0.18)
plt.gcf().subplots_adjust(bottom=0.18)
plt.savefig('h2_td_den_stretched.pdf')
```

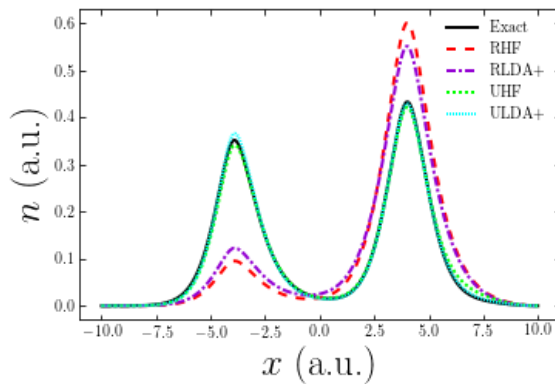

We will now plot the current densities at the end of the simulation:

```
In [37]: # import currents
i = 59
I_ext = pickle.load(open('outputs/h2_{0}/raw/td_ext_cur.db'.format(i), 'rb'))
I_uhf = pickle.load(open('outputs/h2_{0}/raw/td_uhf_cur.db'.format(i), 'rb'))
I_rhf = pickle.load(open('outputs/h2_{0}/raw/td_rhf_cur.db'.format(i), 'rb'))
I_uldap = pickle.load(open('outputs/h2_{0}/raw/td_uldap_cur.db'.format(i), 'rb'))
I_rldap = pickle.load(open('outputs/h2_{0}/raw/td_rldap_cur.db'.format(i), 'rb'))
```

```
In [38]: # system the stretched length
i = 44

# plot currents
plt.plot(x, I_ext[-1,:], linestyle='-', dashes=(), color='k', linewidth=2, label='Exact')
plt.plot(x, I_rhf[-1,:], linestyle='--', dashes=(3, 3), color='red', linewidth=2, label='RHF')
plt.plot(x, I_rldap[-1,:], linestyle='--', dashes=(3,1,1,1), color='darkviolet', linewidth=2, label='RLDA+')
plt.plot(x, I_uhf[-1,:], linestyle='--', dashes=(1, 1), color='lime', linewidth=2, label='UHF')
plt.plot(x, I_uldap[-1,:], linestyle='--', dashes=(0.5,0.5), color='cyan', linewidth=2, label='ULDAP+')

# configure and save plot
plt.legend(frameon=False)
plt.xlabel(r'$x$ (a.u.)', size=25)
plt.ylabel(r'$I$ (a.u.)', size=25)
plt.tick_params(top='on', right='on')
plt.tick_params(direction='in')
plt.gcf().subplots_adjust(left=0.18)
plt.gcf().subplots_adjust(bottom=0.18)
plt.savefig('h2_td_cur_stretched.pdf')
```

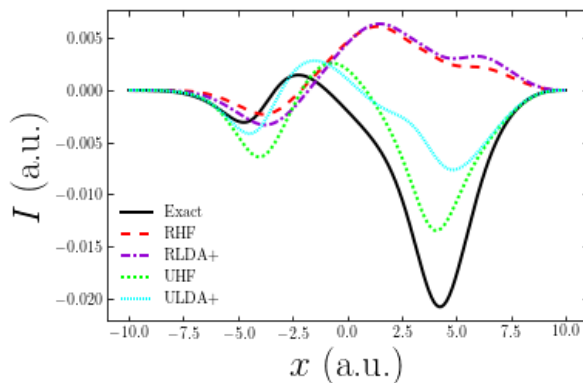

## 7. Features of the exact $V_c$

We will now look at the exact  $V_c$  and both RHFKS and UHFKS at the natural length, and fully stretched length:

```
In [39]: import iDEA.RHFKS
import iDEA.UHFKS
```

```
In [40]: # WARNING: Long Run! Does not need to be run again for rest of the script to work!

# first at the natural length
d = ds[E.argmax()]
i = E.argmax()
pm.run.time_dependence = False
pm.space.v_ext = np.copy(v(x)) # set the external potential
pm.run.name = 'h2_{0}'.format(i)
result_rhfks = iDEA.RHFKS.main(pm, 'ext')
result_uhfks = iDEA.UHFKS.main(pm, 'ext')
```

```
In [41]: i = E.argmax()
vc_rhfs_natural = pickle.load(open('outputs/h2_{0}/raw/gs_extrhfs_vc.db'.format(i), 'rb'))
vc_uhfs_natural = pickle.load(open('outputs/h2_{0}/raw/gs_extuhfs_vc.db'.format(i), 'rb'))

# plot energy curve
plt.plot(x, vc_uhfs_natural+0.027, linestyle='-', color='lime', linewidth=2, label='UHFKS')
plt.plot(x, vc_rhfs_natural-0.005, linestyle=':', color='red', linewidth=2, label='RHFKS')

# configure and save plot
plt.legend(frameon=False)
plt.xlabel(r'$x$ (a.u.)', size=25)
plt.ylabel(r'$V_{\mathrm{c}}$ (a.u.)', size=25)
plt.tick_params(top='on', right='on')
plt.tick_params(direction='in')
plt.gcf().subplots_adjust(left=0.18)
plt.gcf().subplots_adjust(bottom=0.18)
plt.savefig('exact_vc_natural.pdf')
```

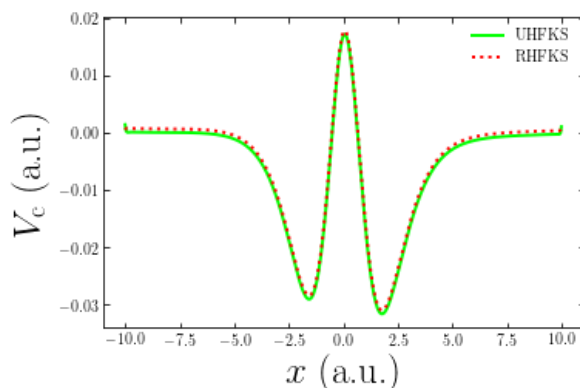

```
In [42]: # WARNING: Long Run! Does not need to be run again for rest of the script to work!

# then at the stretched length
d = ds[53]
print('d = {}'.format(d))
i = 53
pm.run.time_dependence = False
pm.space.v_ext = np.copy(v(x)) # set the external potential
pm.run.name = 'h2_{0}'.format(i)
pm.hfks.mu = 0.01 # stability parameters
pm.hfks.p = 0.05 # stability parameters
pm.hf.nu = 0.1 # stability parameters
result_rhfs = iDEA.RHFKS.main(pm, 'ext')
result_uhfs = iDEA.UHFKS.main(pm, 'ext')
```

```
In [43]: i = 53
vc_rhfks_stretched = pickle.load(open('outputs/h2_{0}/raw/gs_extrhfks_vc.db'.format(i), 'rb'))
vc_uhfks_stretched = pickle.load(open('outputs/h2_{0}/raw/gs_extuhfks_vc.db'.format(i), 'rb'))

# plot energy curve
plt.plot(x, vc_rhfks_stretched, linestyle=':', color='lime', linewidth=2, label='RHFKS')
plt.plot(x, vc_uhfks_stretched, linestyle='-', color='red', linewidth=2, label='UHFKS')

# configure and save plot
plt.legend(frameon=False)
plt.xlabel(r'$x$ (a.u.)', size=25)
plt.ylabel(r'$V_{\mathrm{c}}$ (a.u.)', size=25)
plt.tick_params(top='on', right='on')
plt.tick_params(direction='in')
plt.gcf().subplots_adjust(left=0.18)
plt.gcf().subplots_adjust(bottom=0.18)
plt.savefig('exact_vc_stretched.pdf')
```

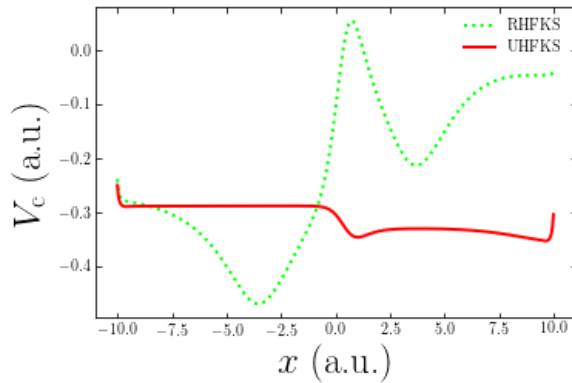

Supplement: Supplementary file 2 [file results_asym.pdf]
